# Supplementary material for: Donor Retention in Online Crowdfunding Communities: A Case Study of DonorsChoose.org
Source: arXiv:1503.02729 source file (2015-03-09)
Supplement: Supplementary file 1 [file 090appendix.tex]

% !TEX root = lidif.tex

\begin{itemize}
	\item ...
\end{itemize}
